# Supplementary material for: Exploiting Frequency Correlation for Hyperspectral Image Reconstruction
Source: arXiv:2406.00683 source file (2024-06-02)
Supplement: Supplementary file 1 [file SDL.tex]

% \begin{table}[tp]
%     \centering
    
%     % \vspace{-0.2cm}
%     % \vspace{}
% \end{table}

\begin{table}[tp]
    % \vspace{-1mm}
    \centering
    \caption{\small The ablation study of the space domain learning.}
    \vspace{-2mm}
    \scalebox{0.79}{
        \label{tab:sdl}
        \begin{tabular}{c c c  c c c c}
        
        		%\small
        		\toprule
                    \rowcolor{lightgray}
        		~~Space Domain Learning~~ & ~~Params $(M)$~~ & ~~FLOPs $(G)$~~ & ~~PSNR~~ & ~~SSIM~~\\
        		\midrule
        		\XSolidBrush & 0.40 & 11.53 & 35.37 & 0.938\\
        		\Checkmark  & 0.55 & 16.30 & \bf36.02 & \bf0.952\\
        		\bottomrule
        \end{tabular}
    }
    \label{tab:table2}
    \vspace{-5mm}
\end{table}
