# Supplementary material for: Exploiting Frequency Correlation for Hyperspectral Image Reconstruction
Source: arXiv:2406.00683 source file (2024-06-02)
Supplement: Supplementary file 2 [file dualdomain.tex]

\begin{table}[!htbp]
    \centering
    \scalebox{0.74}{
        \begin{tabular}{c c c  c c c c}
        		%\small
        		\toprule
        		Baseline-1  & SDLB & FDLB & Params$(M)$ & FLOPs$(G)$ & PSNR & SSIM\\
        		\midrule
        		\checkmark  &  &  & 0.75 & 11.53 & 35.37 & 0.938\\
        		\checkmark  & \checkmark &  & 1.00 & 15.70 & 36.30 & 0.957\\
        		\checkmark  & \checkmark & \checkmark & 1.75 & 21.39 & \bf37.64 & \bf0.966\\
        		\bottomrule
        \end{tabular}
    }
    \vspace{-0.2cm}
    \caption{\small Break-down ablation of two domain learning branches.}
    \label{tab:table3}
    \vspace{-0.2cm}
\end{table}
